# Supplementary material for: Spontaneous rolling on a 90 degree incline
Source: arXiv:2411.18840 ancillary file (2024-11-28)
Supplement: Supplementary file 1 [file supplementary.pdf]

## Supplementary Information: Spontaneous rolling on a 90° incline

Surjyasish Mitra<sup>1</sup>, A-Reum Kim<sup>2</sup>, Boxin Zhao<sup>2</sup>, and Sushanta K. Mitra<sup>1,\*\*</sup>

<sup>1</sup>Department of Mechanical and Mechantronics Engineering, Waterloo Institute for Nanotechnology, University of Waterloo, 200 University Avenue West, Waterloo, ON N2L 3G1, Canada

<sup>2</sup>Department of Chemical Engineering, Waterloo Institute for Nanotechnology, University of Waterloo, 200 University Avenue West, Waterloo, ON N2L 3G1, Canada

**\*\*Corresponding author:** skmitra@uwaterloo.ca

Within this Supplementary Material, we present additional experimental details like PAAm and PDMS fabrication and rheology, static measurements, and image processing. We also provide detailed derivation of the torque created due to contact asymmetry.

### Fabrication of PAAm

To prepare the elastic spheres, we used acrylamide (AAm) as the monomer, N,N'-Methylene-bis-acrylamide (BIS) as the crosslinker, and 2,4,6-tri-methyl benzoyl-diphenylphosphine oxide (TPO) nanoparticle as the initiator (Step 1, Fig. S1). To prepare the TPO nanoparticles, we dissolved 2.5 wt. % of diphenyl (2,4,6-trimethylbenzoyl) phosphine oxide ( $M_w = 348.48$ ), 3.75 wt. % of polyvinylpyrrolidone, and 3.75 wt. % of dodecyl surface sodium salt (SDS) in DI water. We then sonicated the mixture for 5 min at 95°C to obtain 10 wt. % of TPO nanoparticles in DI water. We prepared the pregel solutions by diluting the monomer (4 – 30.0 wt. %), 1 wt. % of the crosslinker (based on the monomer), and 2.5 wt % of TPO nanoparticles (based on the monomer) in 0.5 mM NaIO<sub>4</sub> solution, which acts as the oxygen scavenger. Consequently, we suspended 4  $\mu$ L of the pregel solution in a beaker with n-octane and silicone oil (phenylmethylsiloxane-dimethylsiloxane copolymer, 500 cSt, Gelest), with a 1:2 volumetric ratio between the two to prepare the PAAm spheres. The spherical shapes of the PAAm were obtained by utilizing the density gradient between n-octane (density  $\rho = 0.71$  g/cm<sup>3</sup>) and the silicone oil ( $\rho = 1.08$  g/cm<sup>3</sup>). To do so, we poured the heavier silicone oil in a beaker first and then slowly poured octane on top of the oil (Step 2, Fig. S1). A bi-layer solvent with a smooth density gradient was achieved after a wait time of 1 hour (Step 3, Fig. S1). Following that, we pipetted 4  $\mu$ L of the PAAm pregel solution in the middle of the two solvents (Step 4, Fig. S1) and subsequently cured it under UV light ( $\sim 365$  nm) for 20 min (Step 5, Fig. S1). We rigorously washed the cured PAAm spheres with heptane before use (Step 6, Fig. S1).

### Rheology characterization of PAAm

The elastic properties of the PAAm spheres/drops were characterized using a dynamic shear rheometer (Kinexus Rotational Rheometer, Malvern Instruments). For rheology measurements, each PAAm was polymerized in a petri dish with a thickness of 2 mm. The shear storage ( $G'$ ) and loss ( $G''$ ) modulus of the materials were measured by performing a frequency sweep test on the rheometer from 0.01 to 100 Hz at a strain rate of 1 % and a normal force of 1 N (Fig. S2). All measurements were performed at 25°C, using a parallel plate geometry with a 25 mm diameter plate as the test adopter. The measurements are taken after waiting for 10 min to stabilize the polymer. From the measured  $G'$  and  $G''$  values, we calculated the absolute shear modulus  $|G| = \sqrt{G'^2 + G''^2}$ . Consequently, we used the absolute modulus  $G$  at the lowest frequency  $f = 0.01$  Hz to obtain the static shear modulus  $G_{0,1}$ . The elastic modulus is subsequently calculated using the relation  $E_1 = 3G_{0,1}$ , i.e., considering the Poisson's ratio  $\nu = 1/2$  [6].

### Fabrication and characterization of soft substrates

Soft substrates were prepared using two different commercially available polydimethylsiloxane: PDMS, Sylgard 184 and PDMS, Sylgard 527. First, the base and curing agent of Sylgard 184 and 527 were mixed in the manufacturer specified weight ratios of 10:1 and 1:1, respectively. The mixture was then thoroughly stirred,

dessicated to remove trapped bubbles, and finally cured at 85°C for 12 hours. Before use, the cured substrates were kept at room temperature for 2 hours. Using this technique, we prepared soft coatings of 1 mm thickness on underlying glass substrates. The shear storage and loss modulus of the soft materials were measured by performing a frequency sweep test on a dynamic shear rheometer (Kinexus Rotational Rheometer, Malvern Instruments) from 0.01 to 100 Hz at a strain rate of 1 % and a normal force of 1 N (Fig. S3). Here also, from the measured  $G'$  and  $G''$  values, we calculated the absolute shear modulus  $|G| = \sqrt{G'^2 + G''^2}$ . Consequently, we used the absolute modulus  $G$  at the lowest frequency  $f = 0.01$  Hz to obtain the static shear modulus  $G_{0,2}$ . The elastic modulus is subsequently calculated using the relation  $E_2 = 3G_{0,2}$ , i.e., considering the Poisson's ratio  $\nu = 1/2$ . Additionally, we performed atomic force microscopy measurements (Nanoscope, Digital Instruments) on the Sylgard 184, 10:1 PDMS, i.e., the soft substrate on which rolling was observed. Representative AFM measurements are shown in Fig. S13. On average, the arithmetic mean roughness ( $R_a$ ) and the root mean square height ( $R_q$ ) are  $0.76 \pm 0.06$  nm and  $0.95 \pm 0.08$  nm, respectively.

### Imaging experiments and analysis

Static pinned or sliding configurations of PAAm sphere/drops and water droplets on different substrates were observed using conventional shadowgraphy using DSA Kruss' in-built CCD camera coupled with a macro lens, achieving a spatial resolution of 22-25  $\mu\text{m}/\text{pixel}$ . The rolling experiments were performed using shadowgraphy with three different settings. First, lower magnification (1x) recordings were performed using DSA Kruss' in-built CCD camera at 10 frames per second acquisition rate and a spatial resolution of 22-25  $\mu\text{m}/\text{pixel}$ . These recordings have a larger field of view and exhibits the point of dispensing and extended rolling. However, these recordings are not used for extracting key features (advancing/receding edges, velocity, and contact angles) of the rolling dynamics. Second, moderate magnification experiments were performed with a high-speed camera (FASTCAM AX-200, Photron) operating at acquisition rates of 50-60 frames per second and coupled with a 4x microscope objective lens and an adapter tube providing a spatial resolution of 7-8  $\mu\text{m}/\text{pixel}$ . As mentioned in the main text, these experiments provide the optimal spatio-temporal resolution and are thus used for extracting key features of the rolling dynamics. Note that all experiments with microplastics were conducted using this setting. Lastly, higher magnification rolling experiments were performed using a similar configuration albeit with a 10x long-working distance objective lens (Optem), providing a spatial resolution of 2  $\mu\text{m}/\text{pixel}$ . These recordings provide a close up of the advancing and receding edges, but a lower field of view. Again, these recordings are not used for extracting key features of the rolling dynamics.

Image processing was conducted using an edge detection algorithm in Python [1, 2]. Briefly, shadowgraphy rendered the PAAm sphere dark against a bright background. Consequently, we scanned each frame along the line separating the rolling PAAm sphere from the substrate. The first pixel below a threshold intensity value identified the advancing edge position when scanning from the bright background. Similarly, scanning from the opposite direction located the receding edge position. The threshold intensity typically ranged between 70 a.u and 100 a.u, depending on the image acquisition rate and illumination conditions. Dynamic contact angles at the advancing and receding edges were determined using either a tangent fit or a first-order polynomial fit. To identify the contact asymmetry, a circle was fitted over the PAAm profile to locate its center, and the center's x-coordinate was projected onto the contact interface. Alternatively, the x-coordinate of the outermost advancing point at the central axis can be extracted using edge detection (similar to that performed for advancing/receding edges) and upon subtracting the PAAm sphere's radius, we can identify the center. For rolling experiments without microplastics as markers, a random protrusion or shape irregularity at the periphery of the rolling PAAm sphere is tracked over successive frames to determine angular velocity. Note that multiple experimental runs showed the center-of-mass velocity ranged between 0.46 mm/s and 1.12 mm/s, and the angular velocity ranged between 0.9 rad/s and 2.4 rad/s, respectively.

### Derivation of pressure distribution and torque across the contact interface

We assume two elastic surfaces (say, spheres) with elasticity  $E_1$  and  $E_2$ , and with characteristic length scale  $R$ . The general pressure distribution for symmetric contact of these two elastic surfaces can be expressed as

the superposition of the Hertz problem and the Boussinesq problem [3]:

$$p(r, a, \delta) = p_H \left(1 - \frac{r^2}{a^2}\right)^{1/2} + p_B \left(1 - \frac{r^2}{a^2}\right)^{-1/2} \quad (1)$$

Here,  $a$  and  $\delta$  are the contact radius and indentation depth, respectively. For Hertz [4] or JKR [5] type contacts (Fig. S14a) with symmetric pressure distribution, we have  $p_H = \frac{2aE^*}{\pi R}$  and  $p_B = -\frac{2E^*\delta}{\pi a}$ . By the virtue of symmetry, we have  $p(x, y) = -p(x, y)$  and thus there is no rolling moment about the y-axis (Fig. S14a) since  $M_y = \int \int xp(x, y)dx dy = 0$  [3]. For asymmetric contact, we now have to unequal radii  $a_1$  and  $a_2$  where  $a_1 > a_2$  (Fig. S14b). Unequal contact radii thus changes the Boussinesq part of the solution as,

$$p_B(a) = \frac{E^*}{\pi a} \delta - \frac{1}{2} p_H(a), \quad (2)$$

where the Hertz part of the solution  $p_H(a) = \frac{2aE^*}{\pi R}$  remains unchanged. Thus, the modified general pressure distribution for asymmetric contact can be expressed as ,

$$p(r, a, \delta) = p_H(a) \left(1 - \frac{r^2}{a^2}\right)^{1/2} + \left(\frac{E^*}{\pi a} \delta - \frac{1}{2} p_H(a)\right) \left(1 - \frac{r^2}{a^2}\right)^{-1/2} \quad (3)$$

However, the pressure distribution is different in the two halves of the contact (Fig. S14b) and can be expressed as [3],

$$p(r, a, \delta) = p(r, a_1, \delta), x < 0 \quad (4)$$

$$p(r, a, \delta) = p(r, a_2, \delta), x > 0 \quad (5)$$

The pressure difference due to the two unequal halves generates a moment about the y-axis as [3],

$$M_y = \int_{\pi/2}^{3\pi/2} \int_0^{a_1} xp(r, a_1, \delta) r dr d\phi + \int_{-\pi/2}^{\pi/2} \int_0^{a_2} xp(r, a_2, \delta) r dr d\phi \quad (6)$$

where  $x = r \cos \phi$  and  $y = r \sin \phi$ . Consequently, the moment can be expressed as,

$$M_y = -2 \int_0^{a_1} r^2 p(r, a_1, \delta) dr + 2 \int_0^{a_2} r^2 p(r, a_2, \delta) dr \quad (7)$$

$$= -2 \int_0^{a_1} r^2 \left[ p_H(a_1) \left(1 - \frac{r^2}{a_1^2}\right)^{1/2} + \left(\frac{E^*}{\pi a_1} \delta - \frac{1}{2} p_H(a_1)\right) \left(1 - \frac{r^2}{a_1^2}\right)^{-1/2} \right] dr \quad (8)$$

$$+ 2 \int_0^{a_2} r^2 \left[ p_H(a_2) \left(1 - \frac{r^2}{a_2^2}\right)^{1/2} + \left(\frac{E^*}{\pi a_2} \delta - \frac{1}{2} p_H(a_2)\right) \left(1 - \frac{r^2}{a_2^2}\right)^{-1/2} \right] dr \quad (9)$$

$$= -2 \int_0^{a_1} r^2 \left[ \frac{2a_1 E^*}{\pi R} \left(1 - \frac{r^2}{a_1^2}\right)^{1/2} + \left(\frac{E^*}{\pi a_1} \delta - \frac{1}{2} \frac{2a_1 E^*}{\pi R}\right) \left(1 - \frac{r^2}{a_1^2}\right)^{-1/2} \right] dr \quad (10)$$

$$+ 2 \int_0^{a_2} r^2 \left[ \frac{2a_2 E^*}{\pi R} \left(1 - \frac{r^2}{a_2^2}\right)^{1/2} + \left(\frac{E^*}{\pi a_2} \delta - \frac{1}{2} \frac{2a_2 E^*}{\pi R}\right) \left(1 - \frac{r^2}{a_2^2}\right)^{-1/2} \right] dr \quad (11)$$

$$= -\frac{\pi a_1^3}{4} \left( \frac{2E^*\delta}{\pi a_1} - \frac{a_1 E^*}{\pi R} \right) + \frac{\pi a_2^3}{4} \left( \frac{2E^*\delta}{\pi a_2} - \frac{a_2 E^*}{\pi R} \right) \quad (12)$$

$$= \frac{a_1^2 E^*}{4R} (a_1^2 - 2\delta R) - \frac{a_2^2 E^*}{4R} (a_2^2 - 2\delta R) \quad (13)$$

$$= \frac{E^*}{4R} [(a_1^2 - \delta R)^2 - (a_2^2 - \delta R)^2] \quad (14)$$

$$= \frac{\pi R}{2} (a_1 G_1 - a_2 G_2) \quad (15)$$

where,  $G_1 = \frac{E^*}{2\pi} \frac{(a_1^2 - \delta R)^2}{a_1 R}$  and  $G_2 = \frac{E^*}{2\pi} \frac{(a_2^2 - \delta R)^2}{a_2 R}$  are the strain energy release rates at the receding and advancing edge, respectively.

#### Description of supplementary videos

- **Supplementary movie S1:** Glass sphere falling off. Fall-off of a 1 mm radius glass sphere from a vertical glass substrate. Image acquisition rate is 1000 frames per second and spatial resolution is 7-8  $\mu\text{m}/\text{pixel}$ .
- **Supplementary movie S2:** Sliding water droplet. Sliding of a 1 mm radius water droplet on a vertical glass substrate. Image acquisition rate is 10 frames per second and spatial resolution is 25  $\mu\text{m}/\text{pixel}$ .
- **Supplementary movie S3:** Rolling on a 90° degree incline: Run1. Rolling of a 1 mm radius PAAm 30 wt.% elastic sphere (elasticity,  $E_1 = 169.7 \text{ kPa}$ ) on a vertical PDMS substrate (elasticity,  $E_2 = 2242 \text{ kPa}$ ). Image acquisition rate is 50 frames per second and spatial resolution is 7-8  $\mu\text{m}/\text{pixel}$ .
- **Supplementary movie S4:** Rolling on a 90° degree incline: Run2. Rolling of a 1 mm radius PAAm 30 wt.% elastic sphere (elasticity,  $E_1 = 169.7 \text{ kPa}$ ) on a vertical PDMS substrate (elasticity,  $E_2 = 2242 \text{ kPa}$ ). Image acquisition rate is 50 frames per second and spatial resolution is 7-8  $\mu\text{m}/\text{pixel}$ .
- **Supplementary movie S5:** Rolling on a 90° degree incline: Run3. Rolling of a 1 mm radius PAAm 30 wt.% elastic sphere (elasticity,  $E_1 = 169.7 \text{ kPa}$ ) on a vertical PDMS substrate (elasticity,  $E_2 = 2242 \text{ kPa}$ ). Image acquisition rate is 60 frames per second and spatial resolution is 7-8  $\mu\text{m}/\text{pixel}$ .
- **Supplementary movie S6:** Rolling with microplastics. Rolling of a 1 mm radius PAAm 30 wt.% elastic sphere (elasticity,  $E_1 = 169.7 \text{ kPa}$ ) on a vertical PDMS substrate (elasticity,  $E_2 = 2242 \text{ kPa}$ ) with microplastics dispersed on the substrate. Image acquisition rate is 60 frames per second and spatial resolution is 7-8  $\mu\text{m}/\text{pixel}$ .
- **Supplementary movie S7:** Crack opening and closing. Rolling of a 1 mm radius PAAm 30 wt.% elastic sphere (elasticity,  $E_1 = 169.7 \text{ kPa}$ ) on a vertical PDMS substrate (elasticity,  $E_2 = 2242 \text{ kPa}$ ) highlighting the crack opening and closing. Image acquisition rate is 60 frames per second and spatial resolution is 2  $\mu\text{m}/\text{pixel}$ .
- **Supplementary movie S8:** Rolling and stopping. Rolling of a 1 mm radius PAAm 30 wt.% elastic sphere (elasticity,  $E_1 = 169.7 \text{ kPa}$ ) on a vertical PDMS substrate (elasticity,  $E_2 = 2242 \text{ kPa}$ ). Image acquisition rate is 10 frames per second and spatial resolution is 22  $\mu\text{m}/\text{pixel}$ .
- **Supplementary movie S9:** Extended rolling. Rolling of a 1 mm radius PAAm 30 wt.% elastic sphere (elasticity,  $E_1 = 169.7 \text{ kPa}$ ) on a vertical PDMS substrate (elasticity,  $E_2 = 2242 \text{ kPa}$ ). Image acquisition rate is 10 frames per second and spatial resolution is 22  $\mu\text{m}/\text{pixel}$ .

- 
- [1] S. Mitra, A.-R. Kim, B. Zhao, and S. K. Mitra, Rapid spreading of yield-stress liquids, [Langmuir](#) **40**, 18968 (2024).
- [2] M. van Gorcum, B. Andreotti, J. H. Snoeijer, and S. Karpitschka, Dynamic solid surface tension causes droplet pinning and depinning, [Phys. Rev. Lett.](#) **121**, 208003 (2018).
- [3] C. Dominik and A. Tielens, Resistance to rolling in the adhesive contact of two elastic spheres, [Phil. Mag. A](#) **72**, 783 (1995).
- [4] H. Hertz, Über die berührung fester elastischer körper, [J. für die reine und Angew. Math.](#) **92**, 22 (1882).
- [5] K. L. Johnson, K. Kendall, and A. D. Roberts, Surface energy and the contact of elastic solids, [Proc. Royal Soc. Lon. A](#) **324**, 301 (1971).
- [6] A.-R. Kim, S. Mitra, S. Shyam, B. Zhao, and S. K. Mitra, Flexible hydrogels connecting adhesion and wetting, [Soft Matter](#) **20**, 5516 (2024).

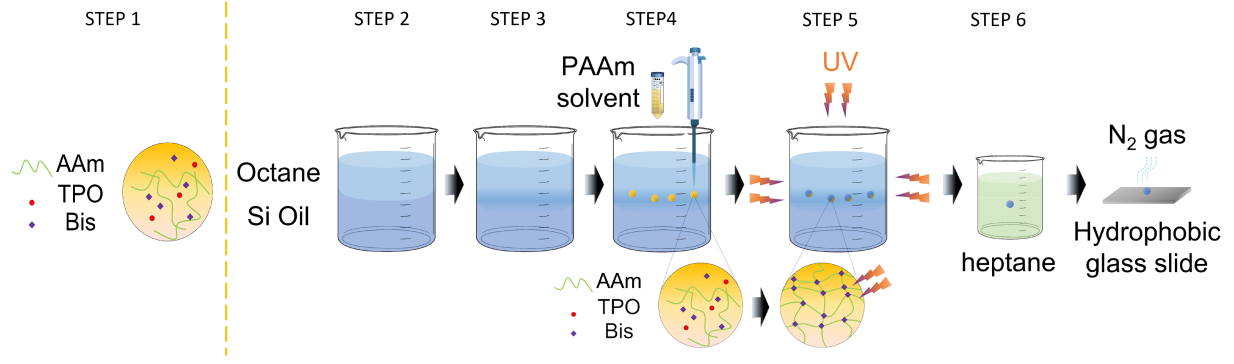

FIG. S1. Schematic showing the different steps of the PAAm elastic spheres/drops preparation procedure. Here, AAm: Acrylamide, TPO: 2,4,6-tri-methyl benzoyldiphenylphosphine oxide, and Bis: N,N'-Methylene-bis-acrylamide. Adapted with permission from Ref. [1].

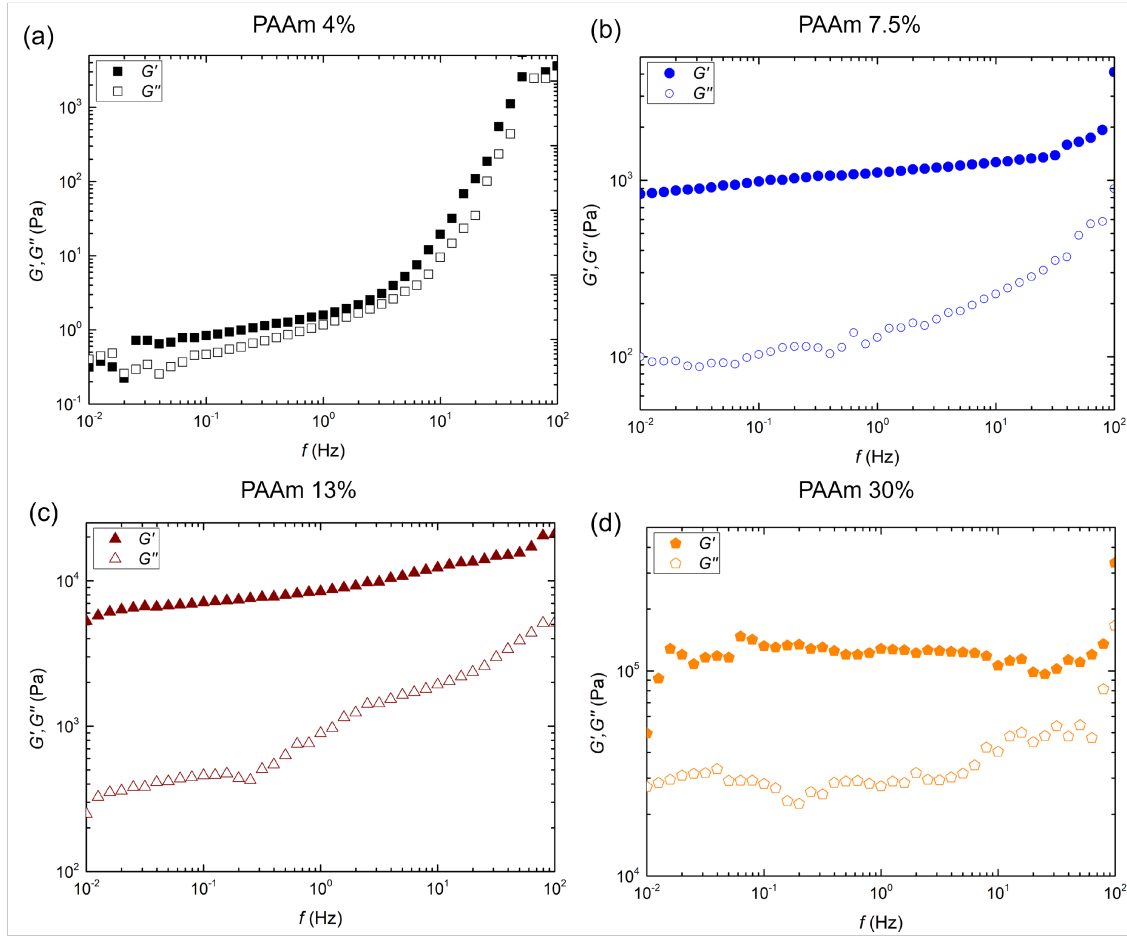

FIG. S2. Variation of shear storage modulus ( $G'$ ) and shear loss modulus ( $G''$ ) with frequency  $f$  for (a) PAAm with 4 wt.% monomer, (b) PAAm with 7.5 wt.% monomer, (c) PAAm with 13 wt.% monomer, and (d) PAAm with 30 wt.% monomer. Subfigure (d) adapted with permission from Ref. [6].

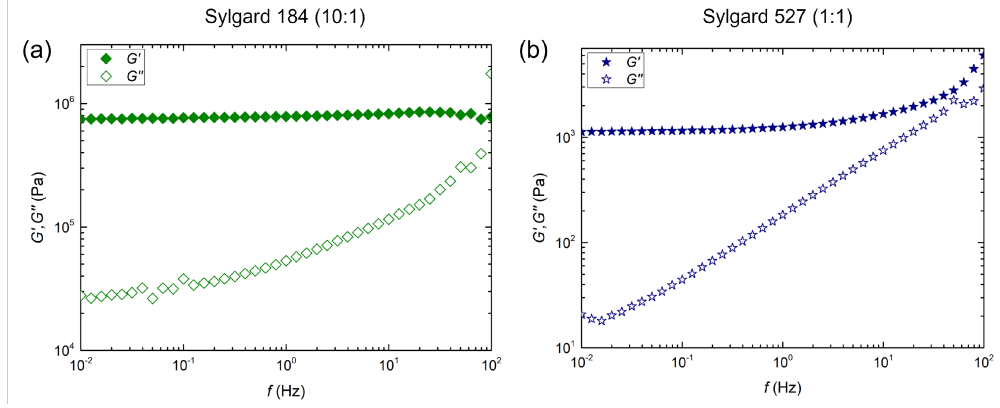

FIG. S3. Variation of shear storage modulus ( $G'$ ) and shear loss modulus ( $G''$ ) with frequency  $f$  for (a) PDMS, Sylgard (10:1) and (b) PDMS, Sylgard 527 (1:1).

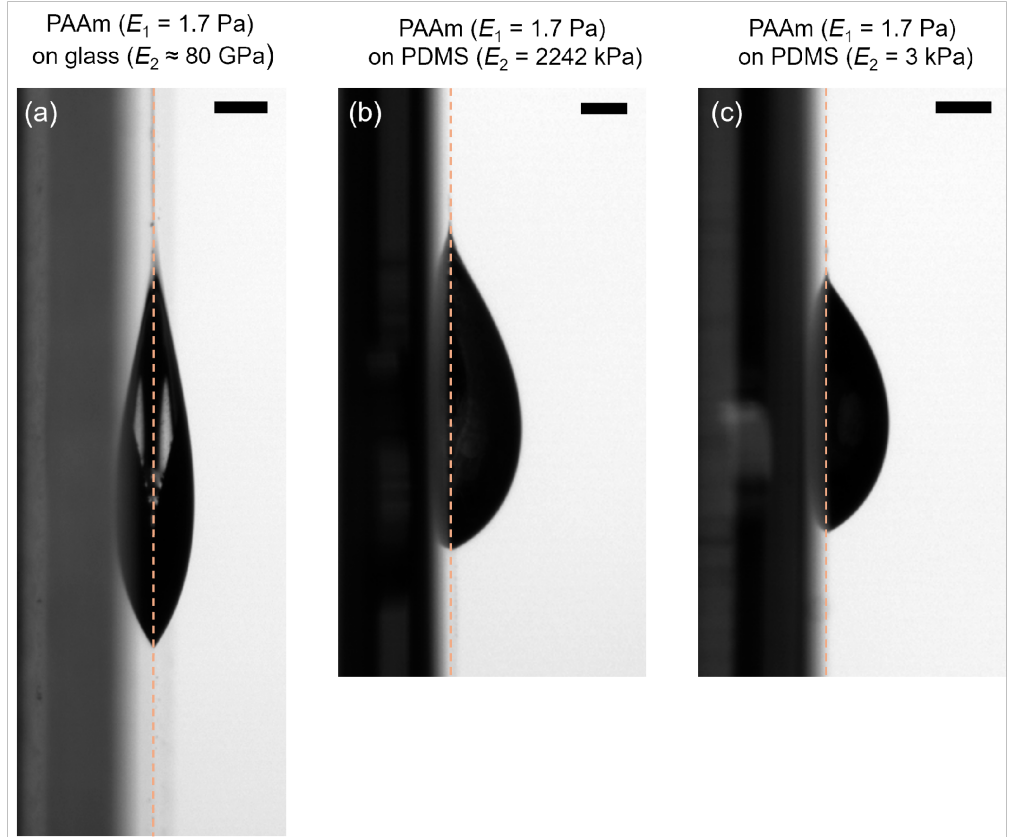

FIG. S4. Static pinned configuration of 1 mm radius PAAm drops with 4 wt% monomers (elasticity,  $E_1 = 1.7$  Pa) on vertical substrates: (a) Glass substrates, (b) PDMS substrates (elasticity,  $E_2 = 2242$  kPa), and (c) PDMS substrates (elasticity,  $E_2 = 3$  kPa). Scale bars represent 1 mm.

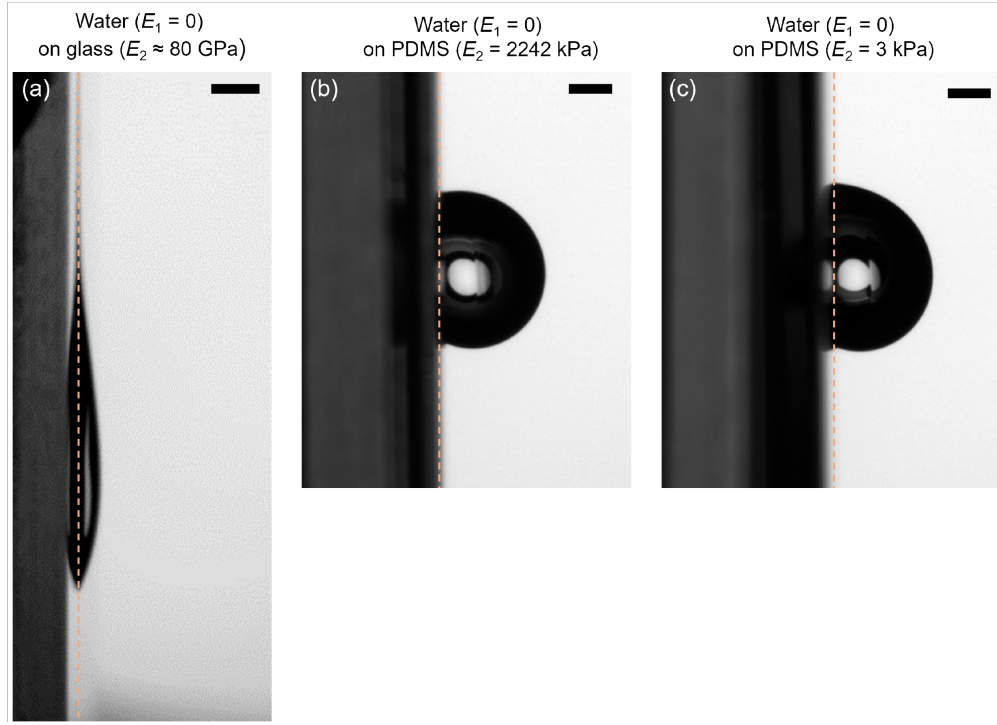

FIG. S5. (a) Snapshot while sliding of a 1 mm radius water droplet on vertical glass substrates. Static pinned configuration of 1 mm radius water droplets on vertical substrates: (b) PDMS substrates (elasticity,  $E_2 = 2242$  kPa) and (c) PDMS substrates (elasticity,  $E_2 = 3$  kPa). Scale bars represent 1 mm.

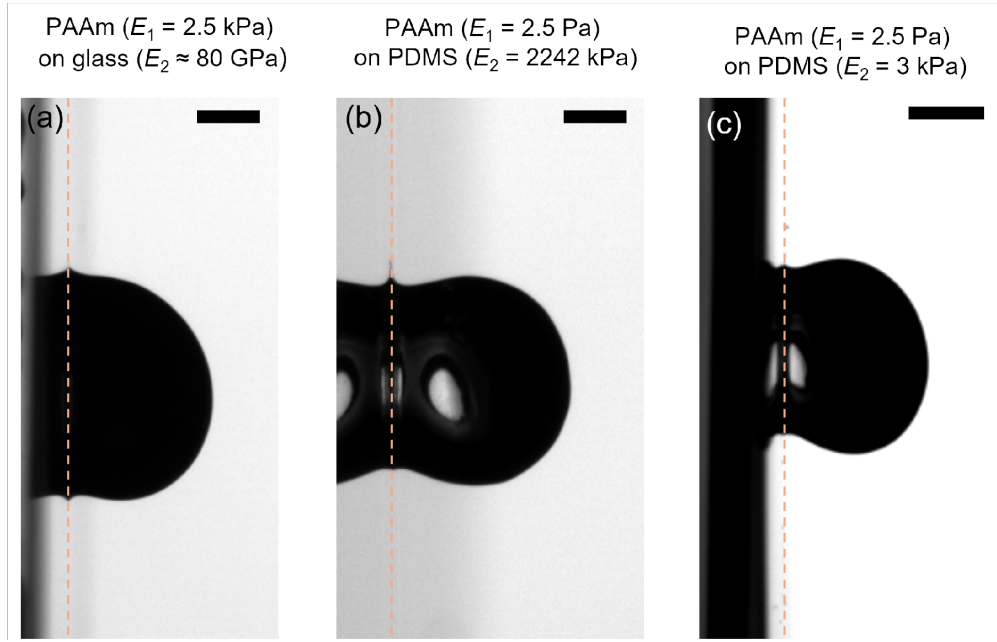

FIG. S6. Static pinned configuration of 1 mm radius PAAm spheres with 7.5 wt% monomers (elasticity,  $E_1 = 2.5$  kPa) on vertical substrates: (a) Glass substrates, (b) PDMS substrates (elasticity,  $E_2 = 2242$  kPa), and (c) PDMS substrates (elasticity,  $E_2 = 3$  kPa). Scale bars represent 1 mm.

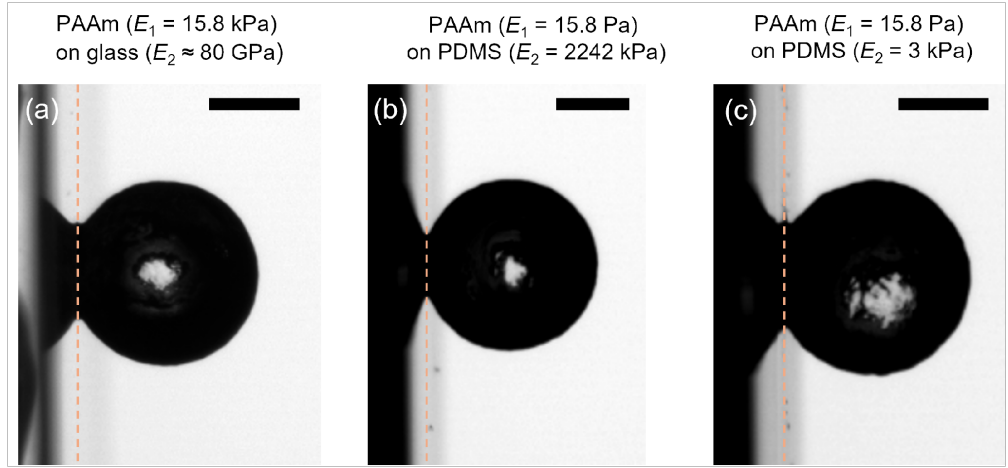

FIG. S7. Static pinned configuration of 1 mm radius PAAm spheres with 13 wt% monomers (elasticity,  $E_1 = 15.8$  kPa) on vertical substrates: (a) Glass substrates, (b) PDMS substrates (elasticity,  $E_2 = 2242$  kPa), and (c) PDMS substrates (elasticity,  $E_2 = 3$  kPa). Scale bars represent 1 mm.

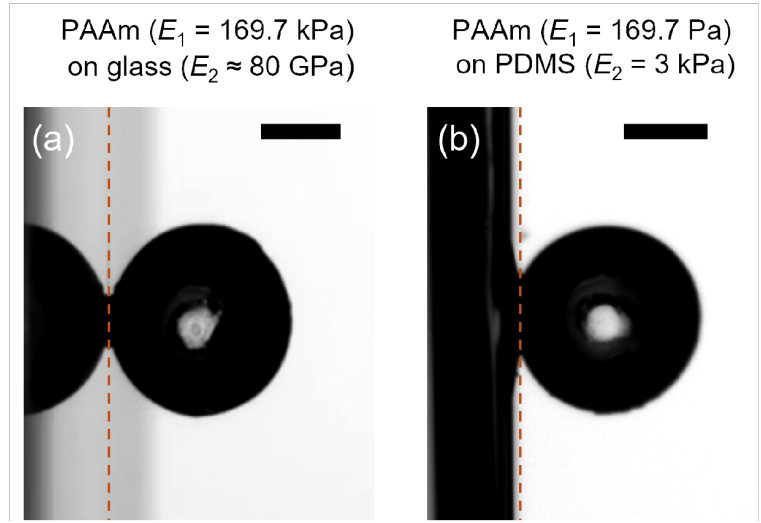

FIG. S8. Static pinned configuration of 1 mm radius PAAm spheres with 30 wt% monomers (elasticity,  $E_1 = 169.7$  kPa) on vertical substrates: (a) Glass substrates and (b) PDMS substrates (elasticity,  $E_2 = 3$  kPa). Scale bars represent 1 mm.

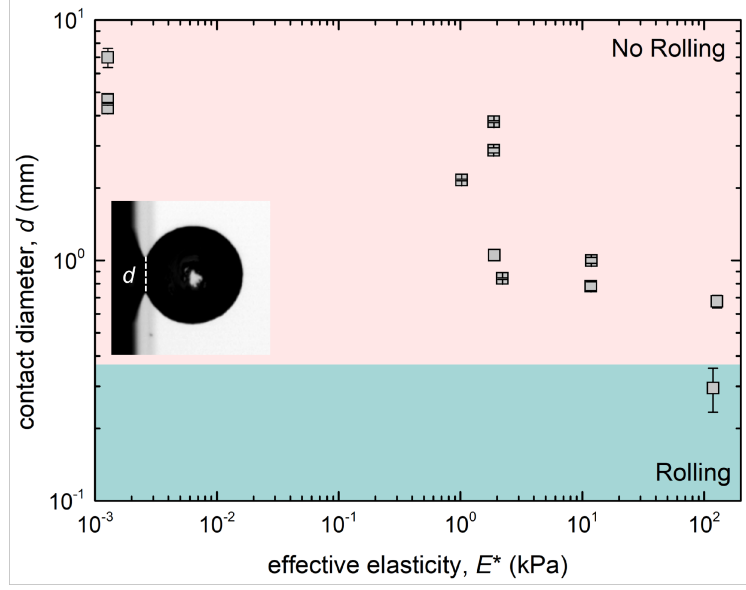

FIG. S9. Variation of contact diameter  $d$  with effective elasticity  $E^*$  for contact of PAAm spheres/drops (elasticity,  $E_1$ ) on soft PDMS substrates (elasticity,  $E_2$ ). Inset shows a representative experimental snapshot highlight the contact diameter  $d$ .

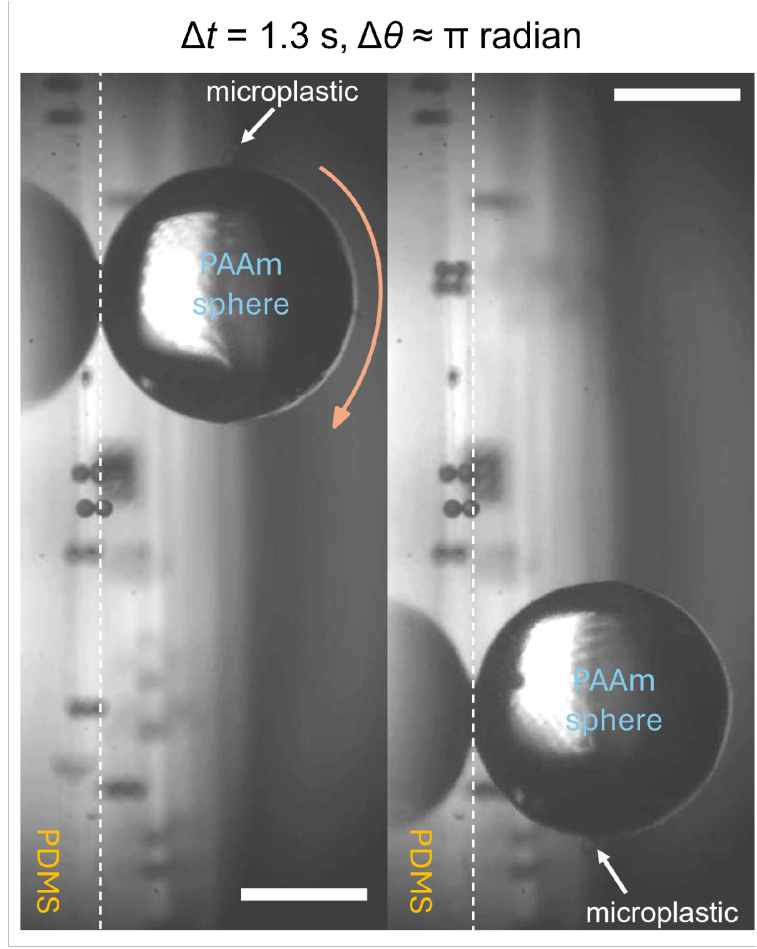

FIG. S10. Experimental snapshots of a rolling event where microplastics are randomly dispersed along the path of the rolling PAAm sphere (elasticity,  $E_1 = 169.7 \text{ kPa}$ ) on PDMS (elasticity,  $E_2 = 2422 \text{ kPa}$ ) substrates. The rolling sphere picks one up along the way which rotates with the sphere. The time interval between the snapshots  $\Delta t = 1.3 \text{ s}$  during which the microplastic has undergone rotation of  $\Delta\theta \approx \pi$  radians leading to angular velocity,  $\omega = \Delta\theta/\Delta t = 2.4 \text{ rad/s}$ . Scale bar represents 1 mm.

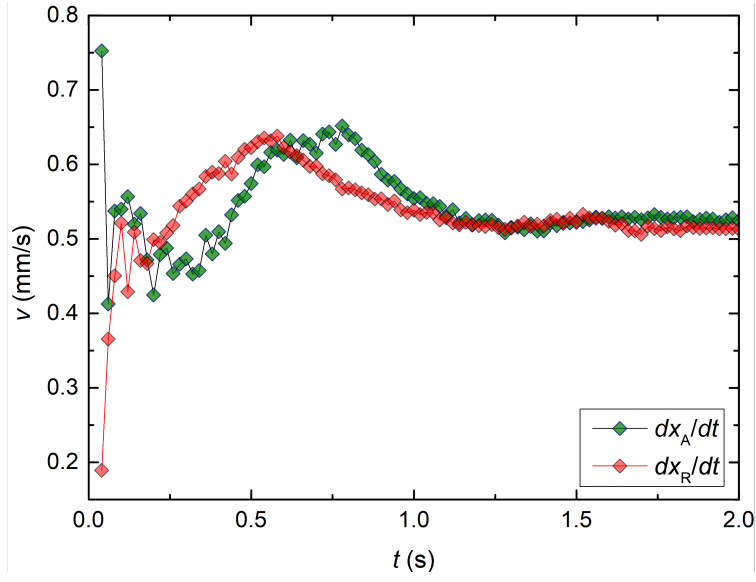

FIG. S11. Evolution of instantaneous velocity  $v$  calculated using finite difference of the advancing ( $dx_A/dt$ ) and receding ( $dx_R/dt$ ) edges during rolling of a PAAm sphere (elasticity,  $E_1 = 169.7$  kPa) on a PDMS substrate (elasticity,  $E_2 = 3$  kPa).

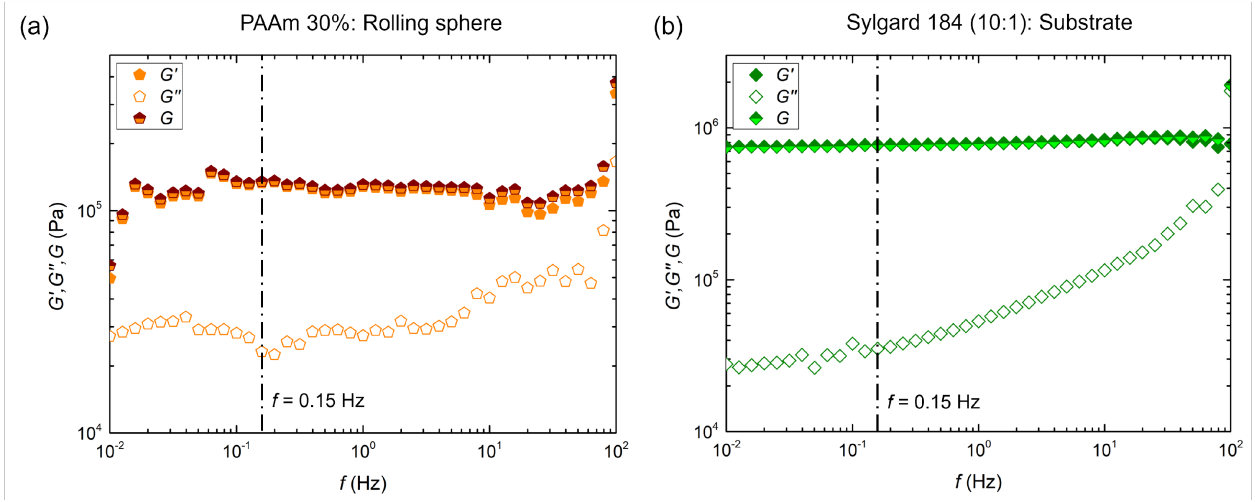

FIG. S12. Variation of shear storage modulus ( $G'$ ) and shear loss modulus ( $G''$ ), and absolute shear modulus  $|G| = \sqrt{G'^2 + G''^2}$  with frequency  $f$  for (a) PAAm with 30 wt.% monomer and (b) PDMS, Sylgard (10:1). The dot-dashed lines show the frequency, i.e.,  $f = 0.15$  Hz at which effective elasticity is considered.

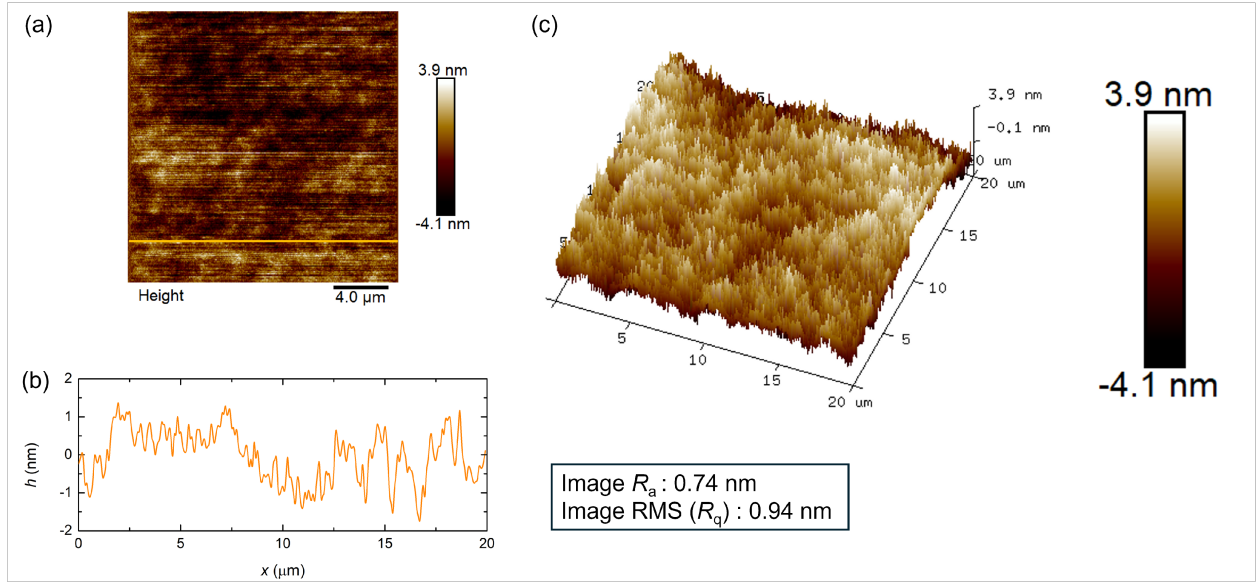

FIG. S13. a) Atomic force microscopy (AFM) scan on a  $20\text{ }\mu\text{m} \times 20\text{ }\mu\text{m}$  cross-section of a Sylgard 184 10:1 PDMS substrate with elastic modulus,  $E_2 = 2422\text{ kPa}$ , i.e., the substrate upon which rolling is observed. (b) Surface profile obtained along the orange line shown in (a). (c) Three-dimensional profile of the entire scan shown in (a).  $R_a$  and  $R_q$  values for the scan are shown.

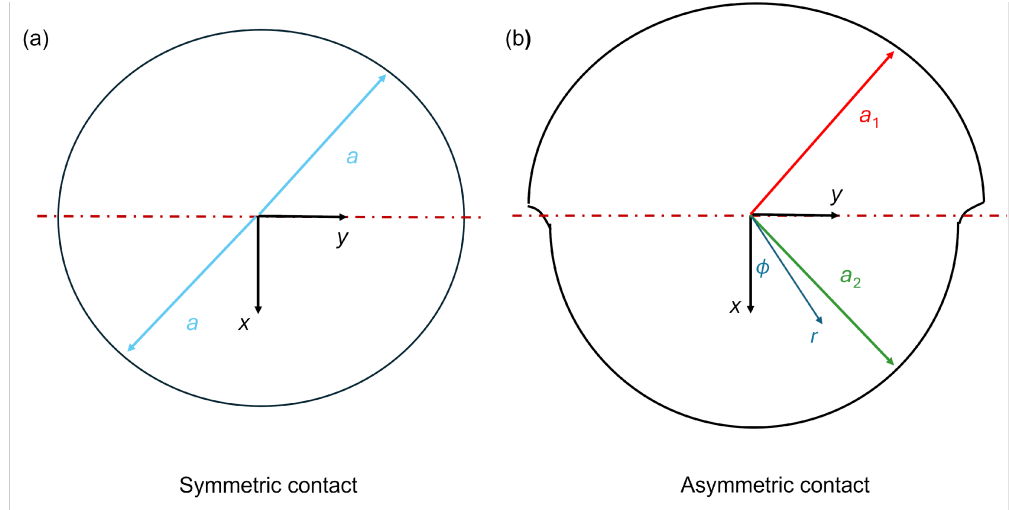

FIG. S14. Bottom-view schematic highlighting (a) symmetric and (b) asymmetric contact configurations.  $a$  is the contact radius for symmetric contact whereas  $a_1$  and  $a_2$  are the contact radii for asymmetric contact.  $r$  and  $\phi$  are the radial and angular coordinates.
